# Supplementary material for: Dial One for Scam: A Large-Scale Analysis of Technical Support Scams
Source: arXiv:1607.06891 source file (2017-03-19)
Supplement: Supplementary file 1 [file appendix.tex]

\appendix

%\section{Sample of Transcribed\\Conversations with Scammers}
%\begin{lstlisting}[basicstyle={\scriptsize\ttfamily},language=English,showstringspaces=false,tabsize=2,frame=tbrl]
%Scammer:	Thank you for calling technical support. How may I assist you?
%Victim:	Hi, good morning. I think I have a problem with my computer because I was browsing the Internet and then it suddenly told me that I was infected with a virus and it asked me to call this number.
%Scammer:	OK. Can you confirm for me, first of all, what Microsoft device you are using?
%Victim:	I am using Windows 7. I do not know if that is what your question is.
%Scammer:	Yeah, that was the question. Windows 7, all right. First of all we will try close that warning page, all right? And we will try to fix the access, all right? And make sure this does not happen again.
%Victim:	OK. I think the warning closed because I think the browser said it had to end the process, so I just wrote the number down before it could close, so ... the site is closed but I am still afraid I have a virus.
%Scammer:	OK. So what you have to do is look at you keyboard. Do you see a Windows button there?
%Victim:	Is it between the Control and ALT?
%Scammer:	Yes, correct.
%Victim:	Yes, I see it.
%Scammer:	You have to press and hold that. You have to press and hold that button. And then press R. R as in Richard, simultaneously.
%Victim:	OK. I did it, yes.
%Scammer:	What do you see now?
%Victim:	I see this little window that says "run."
%Scammer:	All right. Type in there W, W, W, dot. L as in lemon. M as in Mary. I as in indigo. Number one. Dot com.
%Victim:	And should I click OK?
%Scammer:	OK. Yeah.
%Victim:	OK.
%Scammer:	What do you see now? If you see restore option do not click on restore, OK?
%Victim:	OK. I see a page; there is a support connection.
%Scammer:	All right, I am going to generate a six-digit code, OK? You have to type that code into that box. Plus, you have to write it in a paper because this code will be your case number for Microsoft, all right?
%Victim:	OK, I will write it down.
%Scammer:	All right, the code is: 5, 4, 9, 2, 2, 5.
%Victim:	OK, let me type it in. 5, 4, 9--
%Scammer:	Sorry?
%Victim:	I am typing it in.
%Scammer:	It is 5, 4, 9, 2, 2, 5. OK?
%Victim:	I did that. And then what should I do?
%Scammer:	No click on start download.
%Victim:	OK. I did this.
%Scammer:	Now what do you see?
%Victim:	So a download started and it is at the bottom of my Chrome Internet.
%Scammer:	Uh-huh.	You have to double-click on it and run that file, OK?
%Victim:	OK, let me try.
%Scammer:	Uh-huh.
%Victim:	OK. There is a page that opened, a small other window, that says "net creative mind."
%Scammer:	OK, now within 2 seconds you will see some pop-ups on your screen. It will say "Do you want to allow this file?" You have to click on "allow access," "yes," and "OK," all right? All the positive things.
%Victim:	OK, so "allow access." OK. Hit "yes."
%Scammer:	One more pop-up will come. You will see my name there: [inaudible 00:03:54]. You have to press "OK" there.
%Victim:	OK. Give me one second.
%Scammer:	Yeah, it will come in five seconds, all right?
%Victim:	OK.I see your name. Now I see the dialogue. So I should click "OK" on this?
%Scammer:	Yeah. All right, can you see I am moving this now?
%Victim:	Yes.
%Scammer:	OK, I have access. Now let me check what is going on, OK? I am going to close this.
%Victim:	Right. Thank you.
%Scammer:	And, can you tell me, how old is this computer?
%Victim:	It is about 2 and a half years if I am not mistaken.
%Scammer:	And this is your personal computer?
%Victim:	Yes.
%Scammer:	Or multiple users?
%Victim:	I use it but my neighbor also uses it sometimes if their computer is not working.
%Scammer:	OK, what is your full names?
%Victim:	Nathan Sanders.
%Scammer:	Can you spell that?
%Victim:	Yes.
%Scammer:	What was your first name?
%Victim:	Nathan. That is: N, A, T, H, A, N. And my last name is Sanders: S, A, N, D, E, R, S.
%Scammer:	Sanders, OK. All right, I am going to first of all check your system, all right?
%Victim:	All right.
%Scammer:	OK, it is Windows 7. Plus, you have a very good [inaudible 00:05:28], 3.19 gigahertz, your RAM is 2GB. Now, all in all, you have a good configuration, but your rating is very low. You received 1 out of 10.
%Victim:	Yeah, yeah, I do not know why.
%Scammer:	But this configuration it can be more faster. Has this computer slowed down recently?
%Victim:	Yes. Yeah, slowly. I mean, you know, over the months it is becoming more slower.
%Scammer:	OK. OK. I am going to check into it, why it is happening, OK. You will see a black box now.
%Victim:	Yes, I see it.
%Scammer:	Now this thing is going to scan. This is your command prompt. This thing is going to scan your driver, all of the bio section, and most important your network area.
%Victim:	Uh-huh.
%Scammer:	This might take a little bit of time, so I need your patience, all right?
%Victim:	OK.
%Scammer:	Thank you. And can you confirm for me what kind of browsing do you do? Do you do online shopping?
%Victim:	Yeah, occasionally. I mean, you know, I check the news, I check the mail, and sometimes I buy something.
%Scammer:	OK. OK. And do you often witness online advertisements popping up every single time on your browser?
%Victim:	Yes, I do. I do, I do.
%Scammer:	OK. Now that is happening because, first of all, you are not using any protection in your computer. There is no protection. No firewall protection, no anti-virus protection, no network protection, and most important no pop-up protection. And that is what is happening in your computer. What is happening is a lot of viruses are coming and going because there is no protection, right? And I see a lot of junk files stored into your computer.
%Victim:	I see. 	Yeah, I see a lot of things going through this thing but I do not know what they are.
%Scammer:	A lot of them are junk files. These IP areas, you know? IP address areas. [inaudible 00:07:40] your network area. OK, the scan has completed.[inaudible 00:07:49]. The second one says network issue. OK, apart from this device, do you have any other device available?
%Victim:	No, not really.
%Scammer:	[inaudible 00:08:04]
%Victim:	No. That is my only computer.
%Scammer:	Do you have any WiFi devices?
%Victim:	I do not really know what is WiFi. I connect to the Internet, and I pay AT&T for it.
%Scammer:	OK, OK. All right. Now all these errors and warnings are coming from your registry. You see it says "viruses detected; system at risk."
%Victim:	Oh, wow. That is...wow. OK.
%Scammer:	It is confirmed that virus is detected, OK? Now we will be going on into your registry area. I am going to [inaudible 00:08:43]. Now this is also the reason why your computer is also slowing down day by day, right? And viruses are coming in. You do a lot of office work, right?
%Victim:	Yes.
%Scammer:	Word documents in your computer.
%Victim:	Yeah.
%Scammer:	Mm-hmm.	OK, do you see this page?
%Victim:	Mm-hmm.
%Scammer:	This is your registry area, OK? Let us see what is going on. This might also take a little bit of time, OK? So just ... Oh my god. Wow.
%Victim:	What happened?
%Scammer:	All right, do you see this number them: 69?
%Victim:	Yes.
%Scammer:	You have more than 50 errors in warning in your computer stored in [inaudible 00:09:36]. Most of them are critical, you see?
%Victim:	I see. I guess that is bad. I do not really know.
%Scammer:	And it has been in your computer from 2014. It took a little pause, right? It took a little pause, but it started again.
%Victim:	Right.
%Scammer:	You see? And that is how hacking works. A lot of potential hacking processes going on. You see this [inaudible 00:10:00] event?
%Victim:	Mm-hmm, I do.
%Scammer:	This is potential hacking. Now, it means that this device, and your network, is compromised, OK? Which further means that if you have done any online shopping or any online [inaudible 00:10:16] and if you have shared any details, it can be easily hacked, right? Plus, you have a lot of rough files in folders. It can not be deleted because that is how hacking works. They just play with the computers, right? And the most important thing is that you can not delete that, you see? There is no option to delete them successfully.
%Victim:	Right.
%Scammer:	They just multiply every single time, and because of these errors ... [inaudible 00:10:49] critical issue. What is happening is a lot of your Microsoft services are stopping by itself. You are not stopping them but they are stopping, see?
%Victim:	I see.
%Scammer:	Stop, stop.
%Victim:	Yeah, that is true. I see.
%Scammer:	Stop, stop, stop. A lot of them. And most of them are ... yeah, and most of them, you notice, are Microsoft. Now you can imagine that if Microsoft service are not running, your Windows will suffer, right? Because they are the same product.	Now, that is why your computer is slowing down and because you do not have protection, you have virus in your computer. You do not have an IP router so we are having an identity threat issue right now, OK? So we have to block your IP so that it is not visible, all right? So in the future this thing does not happen again, all right?
%Victim:	OK.
%Scammer:	So what we will do is we will transfer this session to our level-three people, OK? Level-three tech guys. I am the level-one. It will be transferred to the level-three guys, and once they have the access they will, first of all, install some software into your computer, right? Because you can see we can not delete them manually, neither can you run the service. You see? You can not enable it manually.
%Victim:	Right.
%Scammer:	So they will install them and the first thing they will do is make this number 0, and make your device, your network, your identity secure, OK? Second thing: running all the services that can not start. You will run them, and the final thing would be removing junk files from your browser and from your storage area, OK? These are the three whole things which our tech guys will work on.
%Victim:	I see.
%Scammer:	And this might take around 14 to 15 minutes, OK?
%Victim:	OK. Is that the service from Microsoft, or--how does it work?
%Scammer:	Yeah. Yeah, this is the Microsoft technical floor. We will transfer it to the level-three people, OK?
%Victim:	OK.
%Scammer:	And they will work on it, and they will complete it. But, Nathan, I have to tell you before transferring it that there will be a charge in it, right? I hope you understand that because, first of all, you have no warranty, second of all, you have no protection, and, third of all, it is an identity threat issue, OK?
%Victim:	I see, yeah.
%Scammer:	Yeah, yeah. So if you just want to go over the fixing it would be 99 dollars. We will remove all these errors and warnings, add a blocker, and remove all junk files and run all the services, OK? But, Nathan, I would strongly recommend you--with fixing--go with a year support or so, right? Because in the year support, first thing you are getting is an anti-virus, OK? Which is compatible, and it is for a lifetime, which will protect your device from viruses and a lot of malicious things coming from your Internet. It will protect you for a lifetime. Second of all, you will get network security, right? And network security would protect your identity and, most important, your IP. And, third, we will add some proper blockers, so that in the future you do not see those advertisements that you see, right? Every time? They will not happen again.
%Victim:	OK.
%Scammer:	And the fourth thing is that you are getting a one-year warranty and a one-year tech support. And that would be 299, OK?
%Victim:	Oh, OK. I see.
%Scammer:	Yeah. So, do you want to go for a one-time support or a one-year support?
%\end{lstlisting}

%\begin{lstlisting}[basicstyle={\scriptsize\ttfamily},language=English,showstringspaces=false,tabsize=2,frame=tbrl]
%Scammer:	[ringing] Thank you for calling technical support, how can I help you?
%Victim:	Uh, good morning. Um, I think I may have a problem with my computer, because I was just looking at, at the internet and websites and suddenly told me that I am infected. And it asked me to call you. 
%Scammer:	If you can sir, can you just read the error message which you are getting on the screen. 
%Victim:	So it said, 'Warning, you may have been infected with a, with virus' and it said no, don't attempt to remove it by yourself, not that I would know how. Um, and then it asked me to call this number, and then I think the browser closed. It said, you know, 'Does not respond, do you want to close?' And I closed. 
%Scammer:	All right, and so do you have any virus protection or something, to protect your computer?
%Victim:	Um, how, how do I check that?
%Scammer:	Sir, you might have paid someone, for example, through AVG, Norton, Mcafee, Kaspersky-
%Victim:	I see-
%Scammer:	Antivirus companies. 
%Victim:	I, I don't remember-
%Scammer:	Any of them-
%Victim:	When I got it. I don't remember if when I bought the computer there was some offer with it. I haven't really paid for software since I bought my computer. 
%Scammer:	Oh, okay. And so how old is your computer?
%Victim:	It's a bit less than two years old. 
%Scammer:	And which windows are you using, windows 7, 8, or 10?
%Victim:	I believe it's 7. 
%Scammer:	Okay, all right. So, sir, in order fix the issue what I'll do, I'll take the remote access of the computer, we'll check the problems, check the pop ups which you are getting. And sir as there is no security at the moment-
%Victim:	Uh huh.
%Scammer:	Paid security, premium security, so there could be charges as well. Because we will be providing you, in order to fix your computer, [00:02:00] the Microsoft securities, the antivirus provided by the Microsoft. He is the manufacturer. All right?
%Victim:	I see. 
%Scammer:	[inaudible 00:02:09] corporation so there could be charges, all right?
%Victim:	Right. Uh, yeah, I guess so, we - you can tell me I guess how much.
%Scammer:	Uh, sir, if you want to go for the one time fix and 1 year technical support, all right, that is just $99. 
%Victim:	Uh huh. 
%Scammer:	And if you want complete for 1 year package, including network security, Microsoft Tools and Microsoft antivirus, for 1 year, that will cost you $149.99, including all 3 softwares, and the best part is they are by the Microsoft. 
%Victim:	Right.
%Scammer:	Plus the 1 year technical support. And, 1 year technical support means, anything goes wrong in 1 year-
%Victim:	Uh huh.
%Scammer:	Anything, software issues computer related issues you just have to call us and there will be no charge to fix that. All right sir.
%Victim:	Right. Yeah, 
%Scammer:	So that's something, right?
%Victim:	Uh huh.
%Scammer:	Uh huh, sorry. 
%Victim:	I, they are a little bit expensive for my budget, even the- your cheapest option, that's, that's true. I don't know if I need it of course. 
%Scammer:	Then you can go for the 1 time fix, that is $69.99, that is a 1 time fix. 
%Victim:	$69.
%Scammer:	Yes sir. That is a minimum, $69.99, that is a 1 time fix. In that you will get the technical support for 7 days, like anything goes wrong apart from the issue which you have got today, and the issues that you are getting today, we insure that. All right, in future if you get that kind of issue in future-
%Victim:	Uh huh.
%Scammer:	There will be no charge to fix that. But if there are different issues, any kind of different issues- 
%Victim:	Uh huh.
%Scammer:	Then only after 7 days there could be charge, and we would be providing you with the software with that as well. 
%Victim:	I see. 
%Scammer:	And the 1 time fix. 
%Victim:	I see. 
%Scammer:	All right?
%Victim:	All right.
%Scammer:	So shall we proceed, or uh, that's all upon you. 
%Victim:	Yeah. Um, yeah I mean, you know, of course if I need, you know if I really need- if my computer really needs it then I guess I could get the $69.99.
%Scammer:	Yes, exactly. All right, no issue sir. Now, are you in front of the computer?
%Victim:	Yes I am. 
%Scammer:	All right. And, it's a laptop or a desktop?
%Victim:	[00:04:00] It's a desktop. 
%Scammer:	All right, so please look on the keyboard, at the left bottom of the keyboard.
%Victim:	Uh huh.
%Scammer:	And there, do you know how windows, what it looks like-
%Victim:	Yes, four squares-
%Scammer:	Windows button, the start button it looks like the flag, exactly you got it. So you're going to press and hold down that windows button, along with letter R, for Romeo, at the same time all right?
%Victim:	Okay. Yes, I did that. 
%Scammer:	Press both, yes, windows as well as the letter R.
%Victim:	Uh huh. Yes, I got a little window that says 'Run.'
%Scammer:	Just type in there H-H- space-H.
%Victim:	Okay. 
%Scammer:	You did that?
%Victim:	Should I click okay?
%Scammer:	Yes sir. H-H-space-H then click okay. 
%Victim:	Okay, I did that. 
%Scammer:	Now, do you see anything else?
%Victim:	Yes, there's another window in the top right that says, uh, uh-
%Scammer:	[inaudible 00:04:59], this page can not be displayed. 
%Victim:	Yes.
%Scammer:	Can you maximize it?
%Victim:	Yes.
%Scammer:	Please do that. 
%Victim:	Okay. 
%Scammer:	Now sir, on the top left of that window you will see a yellow colored caution mark, with a small logo on it. 
%Victim:	Right. 
%Scammer:	Just click on it.
%Victim:	Okay. 
%Scammer:	And then sir you will see jump to url, just set the second last option over there. 
%Victim:	[inaudible 00:05:29]
%Scammer:	Jump to url.
%Victim:	Yes. Okay. 
%Scammer:	Just click on that jump to url.
%Victim:	I clicked it, and there is another little window now. 
%Scammer:	Okay, now type in there www.-
%Victim:	Yes. 
%Scammer:	Lmi1, like L for Lima, M for Maria, I for Indiana, 1.com.
%Victim:	Click okay?
%Scammer:	Yes sir. [00:06:00] Lmi1.com.
%Victim:	Correct. Uh, okay.
%Scammer:	Now what do you see on the screen sir? 
%Victim:	Uh, let's see. So it's working... Um, says support connection. 
%Scammer:	All right, now let me just generate the code for you, from the Microsoft department. Just be hold, let me get the the code, 6 digit code all right?
%Victim:	Sure. 
%Scammer:	[silence] Sir, I have got the code, please note it down. 
%Victim:	Okay. 
%Scammer:	That is 534-
%Victim:	534, yes-
%Scammer:	128.
%Victim:	Okay. 
%Scammer:	And click on start download.
%Victim:	All right. Should I click on run, or save, or cancel?
%Scammer:	Run it. Sir, run it. 
%Victim:	Okay. It says 'Do you want to run the software, [crosstalk 00:07:24]
%Scammer:	Run the software, yes exactly right. 
%Victim:	Okay. Uh, use account control is enabled on this PC, please click okay-
%Scammer:	All right, you'll click okay. 
%Victim:	And then it says, uh, do you want to allow the following program to make change-
%Scammer:	Allow it sir, allow it. 
%Victim:	Okay. [silence] I [00:08:00] see. There's a little window, it says support session established with technician. 
%Scammer:	All right, now press okay. Press okay over there. 
%Victim:	Okay.
%Scammer:	You will see okay over there, press okay.
%Victim:	I clicked on okay.
%Scammer:	You did that?
%Victim:	Yes. 
%Scammer:	All right now the Microsoft department do have the access of your computer, so just be hold, let me take the access on the different software-
%Victim:	Okay. 
%Scammer:	And do not touch anything meanwhile. 
%Victim:	Sure. 
%Scammer:	Yes, thank you. [silence] All right sir, I do have the access now, do you see the team viewer?
%Victim:	Uh, yes I do. 
%Scammer:	Yes, now this is the software from which I do have the remote access of your computer. Now let me check which antivirus you have at the moment in your computer. Oh, I don't see any of them. 
%Victim:	I see. What does that mean?
%Scammer:	Sir, antivirus means a security virus protection software for your computer. 
%Victim:	I see.
%Scammer:	Don't worry, we will provide you that, all right?
%Victim:	All right.
%Scammer:	You don't have to pay extra. Yes. This is the virus protection, no antivirus, windows update not there.
%Victim:	Right.
%Scammer:	Windows defender is not there. And the first and the foremost thing is network access protection. Network access protection isn't, so it is not running. That is turned off, all right? So this is something, all right? 
%Victim:	Did I turn that off? Or did someone turn it off? I mean, I don't know. 
%Scammer:	Sir, because of the viruses, your network protection has been turned [00:10:00] off. Because of the viruses in the computer. Okay?
%Victim:	I see. 
%Scammer:	This is the reason, that is turned off. And now let me check how many viruses are there, in this computer. 
%Victim:	Uh huh. 
%Scammer:	[silence] Sir do you see that?
%Victim:	Yes I do. 
%Scammer:	These are the viruses in your computer. They are 71! Seriously, that means a lot. 
%Victim:	Wow.
%Scammer:	71. And this is the last an unauthorized connection got that access off your computer. 10:31, I guess a while ago. If it's 12:52-
%Victim:	Right. 
%Scammer:	And it is 10:31. So this is the thing which is going on at the moment, now let me check the services of the computer. Sir, do you see the services have been stopped? Stop, stop, stop.
%Victim:	Yes I do. 
%Scammer:	Yes sir, these are the things that are going on at the moment, so many Microsoft services have been stopped right now on your computer. So there is something actually major, it should be turned on. It should be in running condition. But unfortunately they are not running, they are stopped right now. Okay?
%Victim:	I see. 
%Scammer:	And, and do you see this thing, the [inaudible 00:11:31] agent, that is stopped?
%Victim:	Yes. 
%Scammer:	So this is the main thing actually, if I were to have been, you know. I, if I wanted it to get it turned on from here, let me just scroll it from here. Do you see this network access is not running , that is is off.
%Victim:	Yes, yes. 
%Scammer:	If I wanted to turn it on, then I have to turn it on from here. Here is the option. But unfortunately, it is stopped from here as well. So this is something, all right?
%Victim:	All right.
%Scammer:	Everything has been stopped right now. Let me open the task [00:12:00] manager of this computer, and check the services. Oh, here they are. Let me just make it bigger. Now this is something, so is running, stop, stop, stop, stop, stop, stop, stop. 
%Victim:	Right. 
%Scammer:	Again, some of the services are running, some of the services have stopped right now. So this is something, going on with your computer. That is the reason there are charges upkeeping for the premium securities which I will provide you. All right sir?
%Victim:	Uh huh.
%Scammer:	So let me just scroll it down more, yeah stop, stop, stop, stop, you have a lot of things been going on. So these are the things all right? So now, you want to go for 1 time, all right?
%Victim:	Uh huh. 
%Scammer:	Let me just open, yes, the notepad. Let me generate the computer, generate the problem sheet for you, here it is. And you see that, net framework system failure, and the computer has slow speed, network got compromised, browser got hijacked, that is the reason you are facing the pop ups.
%Victim:	I see. 
%Scammer:	Security is not there, a virus protection security, network is also jammed, that has been compromised. Configuration negatively impacted, and trojans attack [inaudible 00:13:10].
%Victim:	Wow. 
%Scammer:	All right. In order to fix this you need to put three softwares in your computer, that is Microsoft security installation, and Microsoft tools. First one is the antivirus from the Microsoft, all right? And the second one is, the tools to block the pop ups and viruses. And the third one is most- first and foremost thing, that is the network protection requirement, that is not there, all right? We need to put that on the server which you are using-
%Victim:	Uh huh.
%Scammer:	To protect this computer, in order to block all the pop ups in future, and unauthorized connections to your computer, all right?
%Victim:	Uh huh. 
%Scammer:	Here, all right. Now let me just go and write it, 1 time fix, that is $69.9- sir, it's only about $20- it's $30 extra, why you are not going for $99.99? [00:14:00] You'll get 1 year service-
%Victim:	Right. 
%Scammer:	1 year service. So this, it's all upon you. Because I don't have to force you, that's all, you know, that's according to your budget. But, you know, after spending just $30 more, you will get it for 1 year, so this is the benefit you will get. Being a technician I would recommend you-
%Victim:	Right. 
%Scammer:	To go for this, and everything is all upon you.
%\end{lstlisting}
